# Supplementary material for: Restricted Boltzmann Machines as Models of Interacting Variables
Source: arXiv:2103.15917 ancillary file (2021-03-29)
Supplement: Supplementary file 1 [file supplementary_material.pdf]

# SUPPLEMENTARY MATERIAL "RESTRICTED BOLTZMANN MACHINES AS MODELS OF INTERACTING VARIABLES"

## 1 Mathematical Derivations

In this section, we derive the parametrisation of the interaction parameters for the Linear and the Exponential activation function cases which are reported in the paper in Eqs. (18) and (20). We omit the discussion of the other two activation functions studied in the paper since the evaluation of the corresponding interaction parameters is straightforward.

The starting point is the general formula for the interaction parameters derived in the paper which, in the case of a separable potential, can be expressed as

$$I^{(s)}_{k_1,k_2,\dots,k_s} = \sum_{\mu=1}^{M}\sum_{p=0}^{s-1}(-1)^p \sum_{j_1<j_2<\dots<j_{s-p}=1}^{s} K\Big(\sum_{l=1}^{s-p} w_{k_{j_l},\mu}\Big), \tag{1}$$

for any order of interaction $s$, where $K(\cdot)$ is the cumulative generating function, $M$ is the number of hidden nodes of the RBM and $W$ is the $N$-by-$M$ weight matrix connecting visible and hidden nodes. As already described in the paper, the cumulative generating function depends on the activation function and, in the case of a separable potential, it can be easily determined by calculating a one dimensional integral. The cumulative generating functions for all the investigated activation functions are reported as an appendix to the main paper.

### 1.1 Linear activation function

In the Linear activation function case, the cumulative generating function writes as

$$K_\mu(q_\mu) = \frac{q_\mu^2}{2} - q_\mu c_\mu. \tag{2}$$

By substituting this expression in equation (1), we obtain

$$I^{\text{Lin}}_{k_1,k_2,\dots,k_s} = \sum_{\mu=1}^{M}\sum_{p=0}^{s-1}(-1)^p \sum_{j_1<j_2<\dots<j_{s-p}=1}^{s} \left(\frac{1}{2}\sum_{l=1}^{s-p}\sum_{h=1}^{s-p} w_{k_{j_l},\mu} w_{k_{j_h},\mu} - c_\mu \sum_{l=1}^{s-p} w_{k_{j_l},\mu}\right). \tag{3}$$

First, we consider the terms in the brackets involving only single weight parameters, i.e.

$$-\sum_{\mu=1}^{M} c_\mu \sum_{p=0}^{s-1}(-1)^p \sum_{j_1<j_2<\dots<j_{s-p}=1}^{s} (w_{k_{j_1},\mu} + \dots + w_{k_{j_{s-p}},\mu}). \tag{4}$$

By inspecting the inner summation in the above equation, one can realise that the number of times that, for instance, the parameter $w_{k_1,\mu}$ appears is equal to all possible ways of choosing the other $s-p-1$ addends out of the $s-1$ possible weights remaining in the summation after having chosen $w_{k_1,\mu}$. This corresponds to $\binom{s-1}{s-p-1}$ and it is true for all the weights in the sum, so that

$$\sum_{p=0}^{s-1}(-1)^p \sum_{j_1<j_2<\dots<j_{s-p}=1}^{s} \sum_{l=1}^{s-p} w_{k_{j_l},\mu} = \sum_{p=0}^{s-1}(-1)^p \binom{s-1}{s-p-1} \sum_{j=1}^{s} w_{k_j,\mu}. \tag{5}$$

We now introduce the following identity

$$\sum_{p=0}^{q}(-1)^p \binom{q}{q-p} = \delta_q, \tag{6}$$

where $\delta_q$ is the Kronecher delta function which is different from zero and equal to one only for $q = 0$, i.e. $\delta_0 = 1$ [1]. By replacing the identity (6) into equation (5), we find that

$$\sum_{p=0}^{s-1}(-1)^p \sum_{j_1<j_2<\cdots<j_{s-p}=1}^{s} \sum_{l=1}^{s-p} w_{k_l,\mu} = \sum_{p=0}^{s-1}(-1)^p \binom{s-1}{s-p-1} \sum_{j=1}^{s} w_{k_j,\mu} = \delta_{s-1} \sum_{l=1}^{s} w_{k_{j_l},\mu} = \delta_{s-1} w_{k_1,\mu}. \quad (7)$$

Now we analyse the other terms in equation (3) which involve products of two weights. We rewrite those terms by separating the cases in which the two weights are equal from those where the two weights are different

$$\frac{1}{2}\sum_{p=0}^{s-1}(-1)^p \sum_{j_1<j_2<\cdots<j_{s-p}=1}^{s} \left( \sum_{l=1}^{s-p} w^2_{k_{j_l},\mu} + 2 \sum_{l_1<l_2=1}^{s-p} w_{k_{j_{l_1}},\mu} w_{k_{j_{l_2}},\mu} \right). \quad (8)$$

We proceed following the same argument as before: each $w^2_{k_{j_l},\mu}$ in the summation will appear $\binom{s-1}{s-p-1}$ times and each product of the type $w_{k_{j_{l_1}},\mu} w_{k_{j_{l_2}},\mu}$ will instead appear $\binom{s-2}{s-p-2}$ times. By simplifying the summations in equation (8), we get

$$\frac{1}{2}\sum_{p=0}^{s-1}(-1)^p \binom{s-1}{s-p-1} \sum_{j=1}^{s} w^2_{k_j,\mu} + \sum_{p=0}^{s-1}(-1)^p \binom{s-2}{s-p-2} \sum_{j_1<j_2=1}^{s} w_{k_{j_1},\mu} w_{k_{j_2},\mu}. \quad (9)$$

As before, we can now exploit the identity in equation (6)

$$\frac{1}{2}\delta_{s-1} \sum_{j=1}^{s} w^2_{k_j,\mu} + \delta_{s-2} \sum_{j_1<j_2=1}^{s} w_{k_{j_1},\mu} w_{k_{j_2},\mu} = \frac{1}{2}\delta_{s-1} w^2_{k_1,\mu} + \delta_{s-2} w_{k_1,\mu} w_{k_2,\mu}. \quad (10)$$

Finally, by inserting equations (7) and (10) into equation (3), we arrive at the final equation

$$I^{\text{Lin}}_{k_1,k_2,\dots,k_s} = \delta_{s-1} \sum_{\mu=1}^{M} \left( \frac{1}{2} w^2_{k_1,\mu} - c_\mu w_{k_1,\mu} \right) + \delta_{s-2} \sum_{\mu=1}^{M} w_{k_1,\mu} w_{k_2,\mu}, \quad (11)$$

which proves that for $s > 2$, $I^{\text{Lin}}_{k_1,k_2,\dots,k_s} = 0$ and $I^{\text{Lin}}_{k_1,k_2,\dots,k_s} \neq 0$ only for $s = 1$ and $s = 2$ consistently with the result of section 2.1 and Eqs. (18a) and (20a) in the paper.

### 1.2 Exponential activation function

The cumulative generating function of a density which induces an Exponential activation function is

$$K_\mu(q_\mu) = \exp(-c_\mu)(\exp(q_\mu) - 1). \quad (12)$$

By substituting this expression into equation (1) we find that

$$I^{\text{Exp}}_{k_1,k_2,\dots,k_s} = \sum_{\mu=1}^{M} \exp(-c_\mu) \sum_{p=0}^{s-1}(-1)^p \sum_{j_1<j_2<\cdots<j_{s-p}=1}^{s} \left( \exp(\sum_{l=1}^{s-p} w_{k_{j_l},\mu}) - 1 \right). \quad (13)$$

However the latter expression can be significantly simplified by exploiting equation (6). In fact, the constant part in the brackets can be embedded in the summation over $p$ by moving the upper index from $s-1$ to $s$, namely

$$I^{\text{Exp}}_{k_1,k_2,\dots,k_s} = \sum_{\mu=1}^{M} \exp(-c_\mu) \sum_{p=0}^{s}(-1)^p \sum_{j_1<j_2<\cdots<j_{s-p}=1}^{s} \prod_{l=1}^{s-p} \exp(w_{k_{j_l},\mu}), \quad (14)$$

which follows from the fact that

$$\sum_{p=0}^{s-1}(-1)^p \sum_{j_1<j_2<\cdots<j_{s-p}=1}^{s} = \sum_{p=0}^{s-1}(-1)^p \binom{s}{s-p} = -(-1)^s. \quad (15)$$

Finally, it is easy to verify in equation (14) that the inner summations represent the expansion of the product $\prod_{j=1}^{s}(\exp(w_{k_j,\mu}) - 1)$, so that equation (13) becomes

$$I^{\text{Exp}}_{k_1,k_2,\dots,k_s} = \sum_{\mu=1}^{M} \exp(-c_\mu) \prod_{j=1}^{s} (\exp(w_{k_j,\mu}) - 1), \quad (16)$$

as reported in Eqs. (18d) and (20d).

[1] Notice that $\binom{0}{0} = 1$ is well defined and corresponds to the vertex of the Pascal's triangle. Equation (6) is indeed easily verified from the binomial formula.

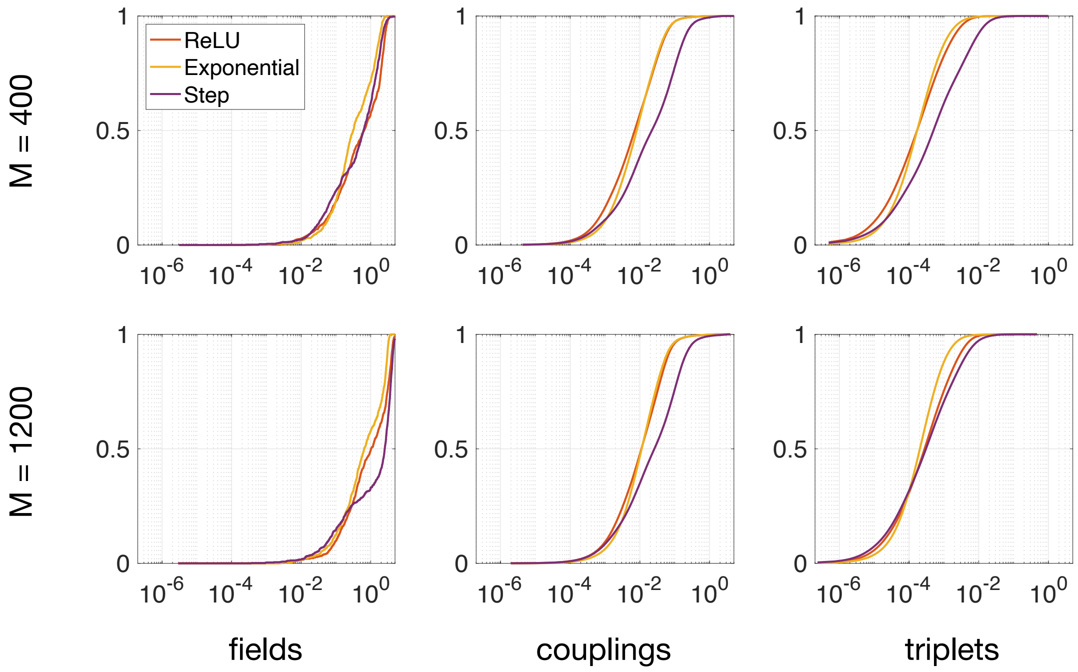


Figure 1: Cumulative distribution of absolute values of interaction parameters induced in RBMs learnt on the MNIST data with different activation functions and with M = 400 (first row) and M = 1200 (second row). The interaction parameters reported are the fields (first column), the pairwise interactions or couplings (second column) and the three-body interactions (third column).

## 2 Supplemental analysis interaction parameter

### 2.1 Distribution of RBM parameters and corresponding interaction parameters

In this section we report the distribution of absolute values of interaction parameters up to the third order which are induced by the RBMs learnt on the MNIST data and described in the main text. In particular we show in Figure 1 the interactions resulting from RBMs with nonlinear activation functions and with $M = 400$ and $M = 1200$ hidden nodes. The figure illustrates that the the cumulative distribution of absolute values of parameters shifts towards smaller values by orders of magnitude as we increase the interaction order, that is proceeding from fields [2] to triplets, and this fact holds true for all activation functions and hidden node numbers reported in the figure. This seemingly exponential decay of the typical magnitude of interaction orders is what we referred in the paper as the hierarchical structure of interactions learnt by RBMs on the MNIST data. Thus Figure 1 complements with more details what reported by Figure 11 in the main text.

As we argue in the paper, this behaviour is consistent with what a small parameter expansion (Eq. 21 in the paper) of the mapping (Eq. 14 in the paper) would predict. Figure 8 and 9 in the paper exhibit evidence supporting the validity of the small parameter approximation. In Figure 2 we report the distributions of absolute values of all RBM parameters: biases on visible nodes, weights and biases on the hidden nodes. Specifically, the distributions of weights (central column) display absolute values that are almost always much smaller than unity which further confirm the small parameter assumption and, thus, further substantiate the result that interaction models learnt by RBMs on the MNIST data are fundamentally low order models with relative importance of interactions decreasing with interaction order. It is also interesting to notice in the figure that some weights are actually left unchanged by the learning procedure, namely those piling up to form vertical segments at $w \sim \sqrt{0.1/N}$.

[2] In order to highlight the effect of the RBM weights on the induced parameters and in order to compare on the same footings fields with other parameters, we have subtracted the bias term contribution to the fields in the plot.

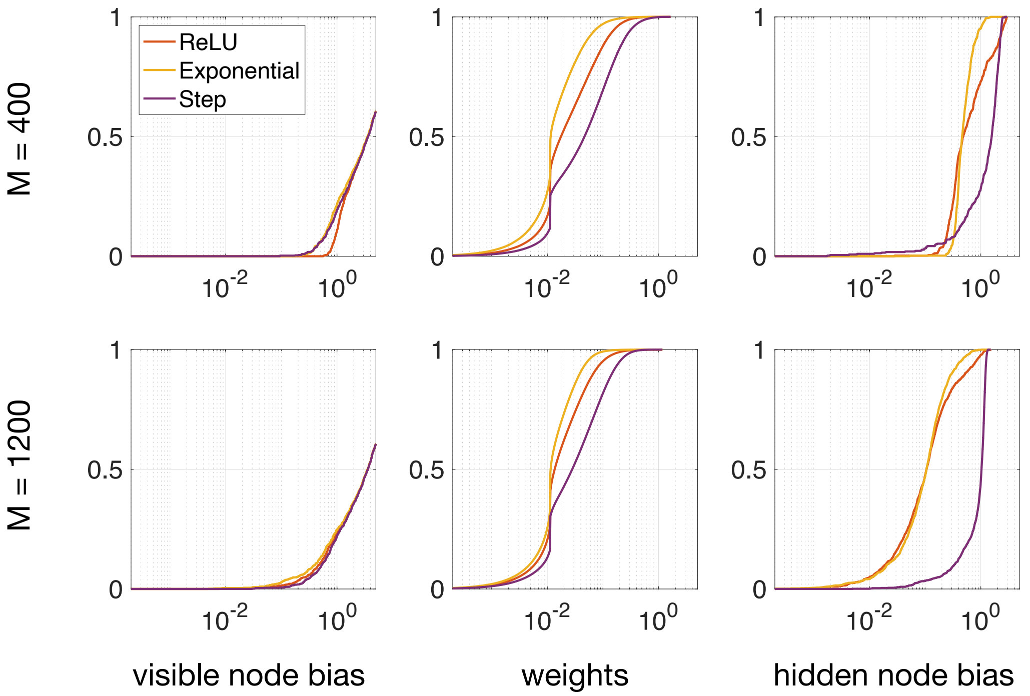


Figure 2: Cumulative distribution of absolute values of RBM parameters learnt on the MNIST data with different activation functions and with M = 400 (first row) and M = 1200 (second row). The parameters reported are the bias on the visible nodes (first column), the weights (second column) and the bias on the hidden nodes (third column).

### 2.2 Comparison interaction parameters learnt on different chunks of MNIST data

In this section we test the robustness of the inferred interaction parameters by comparing interactions up to the third order which are learnt from separate halves of the entire MNIST dataset against the interactions reported in the paper which are inferred instead from the standard MNIST training dataset. In fact, RBMs weights are difficult to compare directly given that the ordering of hidden nodes is unknown and not fixed across RBMs. On the other hand, interaction parameters involve only visible nodes and, as such, they are directly comparable.

In order to perform this comparison we trained RBMs with a ReLU activation function and $M = 400$ hidden nodes on two "balanced" halves of the entire MNIST dataset (70k samples), where each half contains the same number of examples for each digit. The training procedure was the same as that outlined in the main paper with an initial learning rate equal to $0.005$. In all cases, the algorithm achieves a smooth convergence within 500 epochs and no sign of overfitting was detected. In fact, both the pseudo-likelihood and likelihood values of trained models evaluated on the complementary halves show comparable values, as reported in the table below

| | Pseudo-likelihood test set | Likelihood test set |
|---|---|---|
| first half (35k samples) | -60.31 | -87.84 |
| second half (35k samples) | -60.68 | -89.68 |
| standard training dataset (60k samples) | -54.33 | -81.65 |

From the table it is clear that the model trained on the standard dataset achieves larger values of both the likelihood and the pseudo-likelihood function. This is due to the size of the training set which is larger in the standard dataset case (60k samples) as compared to when considering halves of the entire dataset (35k samples each half).

After training we applied the mapping presented in the main text to evaluate the interaction parameters up to the third order. Figure 3 illustrates the results of the comparison among parameters inferred from the two halves and those inferred from the entire training dataset. Interaction parameters are found to be highly consistent across the two halves of the dataset (red circles) with a relative uncertainty increasing with the interaction order, as predicted by analysing Eq. (21) in the main paper. As expected, larger differences are associated with parameters inferred from the entire dataset

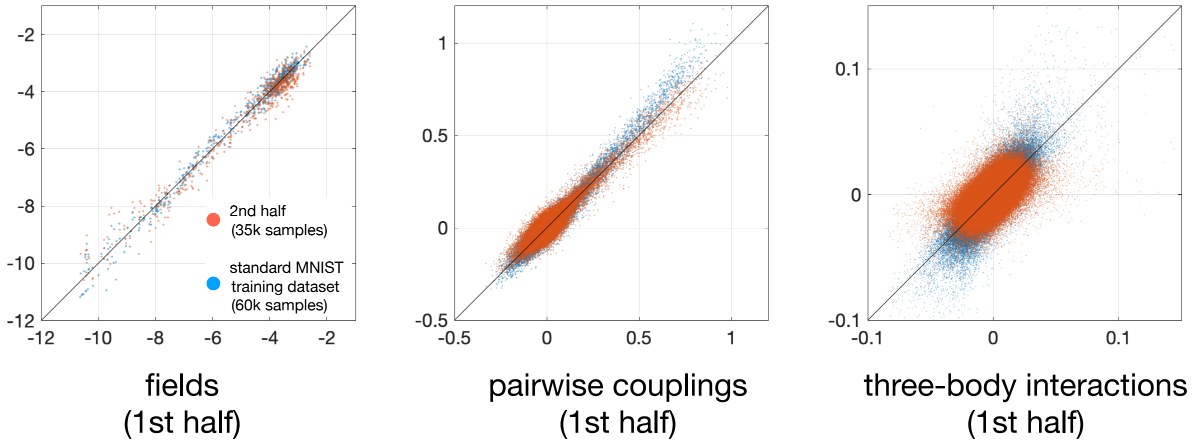


Figure 3: Comparison of interaction parameters up to the third order, that is fields, pairwise and three-body interactions, across the two halves of the "balanced" dataset (red circles) and between the first half and the standard MNIST training dataset (blue circles).

(blue circles). However, these differences amount to a simple rescaling of parameters and look almost always negligible except for the few large parameters.
